# Supplementary material for: A Receding Horizon Push Recovery Strategy for Balancing the iCub Humanoid Robot
Source: arXiv:1705.10638 source file (2017-05-30)
Supplement: Supplementary file 1 [file appendix.tex]

%!TEX root = ../steprecovery.tex
% \appendix
